# Supplementary material for: Finding the stable structures of W$_x$N$_1$$_-$$_x$ with an $ab$$-$$initio$ high-throughput approach
Source: arXiv:1403.2762 source file (2014-03-11)
Supplement: Supplementary file 1 [file supplementary.pdf]

# Supplementary material for "Finding the stable structures of WN with an *ab-initio* high-throughput approach"

Michael J. Mehl*
*Center for Computational Materials Science, Naval Research Laboratory, Washington DC 20375*

Daniel Finkenstadt and Christian Dane
*Department of Physics, U.S. Naval Academy, Annapolis MD 21402*

Gus L. W. Hart
*Department of Physics and Astronomy, Brigham Young University, Provo, UT 84602*

Stefano Curtarolo†
*Materials Science, Electrical Engineering, Physics and Chemistry, Duke University, Durham NC 27708*
(Dated: January 31, 2014)

This is a listing of structures discussed in the main body of the paper, including space groups, lattice constants, Wyckoff positions of atoms, k-point mesh information, energy as computed by VASP, and enthalpy compared to the reference system of $\alpha N_2$ and BCC W.

## I. COMPUTATIONAL DETAILS

All calculations done here used VASP[1–3] with PAW Potentials[4,5] and using the AFLOW automatic framework[6–8]. The general form of INCAR file used was

```
ISYM=2          # SYMMMETRY=ON
IBRION=2        # Relax with conjugate gradient (when appropriate)
PREC=Accurate   # avoid wrap around errors
ENMAX=560       # 1.4*ENMAX (400) of pseudopotentials
LREAL=.FALSE.   # reciprocal space projection technique
EDIFF=1E-6      # high accuracy required
ALGO=Fast       # ALGO = Fast
SYMPREC=1e-7    # Precise Symmetry
ISPIN=1         # SPIN=OFF
ISMEAR=-1       # Fermi broadening
SIGMA=0.0272    # About 0.002 Ry
```

The vdW-DF2[9] functional as implemented in VASP[10,11] was used to study the effect of van der Waals interactions. In this case we used the PBE[12] PAW potentials, and modified the INCAR file to include the lines:

```
LUSE_VDW = .TRUE. # Turn on the van der Waals functional
AGGAC = 0.0000    # Turn off the GGA part of the PBE correlation
GGA = ML          # Use rPW86 exchange
Zab_vdW = -1.8867 # With a parameter change
```

In the following, the line "Mesh" gives the K-point mesh for the final calculations done for each structure. "Γ" indicates that the mesh is centered at the origin, while "M-P" indicates that the Monkhorst-Pack special k-point scheme[13] was used. The final entry on this line is the number of points in the irreducible Brillouin zone of the minimum energy structure.

The line labeled "Energy" gives the converged total energy found by VASP for this structure.

## II. LOCAL DENSITY APPROXIMATION

The following calculations were all done using the local density approximation.

Note that there are two forms for $\alpha N_2$, reflecting the two possible choices for the ground state. Computationally, the two are almost identical in energy. We use the higher symmetry $Pa3$ structure as our reference state.

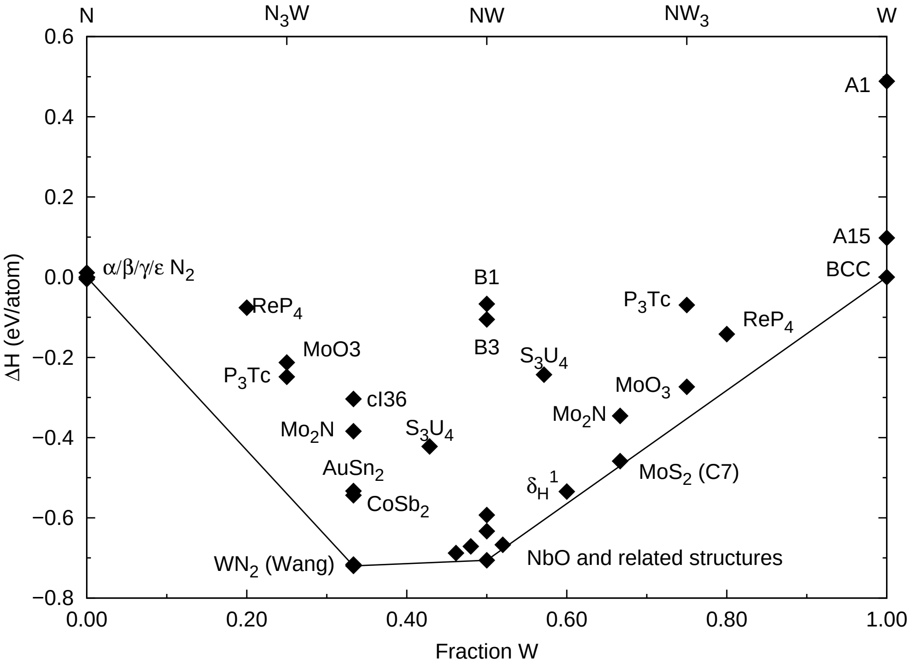


FIG. 1. Enthalpy per atom for $N_{1-x}W_x$ using the Local Density Approximation

1. $\alpha N_2$: High symmetry state:

| | | | |
|---|---|---|---|
| Space Group | $Pa\bar{3}$ | $T_h^6$ | #205 |
| Pearson Symbol | | cP8 | |
| $a$ , $b$ , $c$ | 5.22328Å | 5.22328Å | 5.22328Å |
| $\alpha$ , $\beta$ , $\gamma$ | 90° | 90° | 90° |
| Wyckoff Positions: | | | |
| N (8c) | 0.06094 | 0.93906 | 0.43906 |
| Mesh Γ | 8 × 8 × 8 | 45 pts | in IBZ |
| Energy | | -70.49148 eV | |

2. $\alpha N_2$: Low symmetry state:

| | | | |
|---|---|---|---|
| Space Group | $P2_13$ | $T^4$ | #198 |
| Pearson Symbol | | cP8 | |
| $a$ , $b$ , $c$ | 5.22293Å | 5.22293Å | 5.22293Å |
| $\alpha$ , $\beta$ , $\gamma$ | 90° | 90° | 90° |
| Wyckoff Positions: | | | |
| N (4a) | 0.81097 | 0.68903 | 0.31097 |
| N (4a) | 0.68907 | 0.81093 | 0.18907 |
| Mesh Γ | 16 × 16 × 16 | 249 pts | in IBZ |
| Energy | | -70.49142 eV | |

3. $\beta N_2$:

| | | | |
|---|---|---|---|
| Space Group | $P6_3/mmc$ | $D_{6h}^4$ | #194 |
| Pearson Symbol | | hP4 | |
| $a$ , $b$ , $c$ | 3.54333Å | 3.54333Å | 6.75879Å |
| $\alpha$ , $\beta$ , $\gamma$ | 90° | 90° | 120° |
| Wyckoff Positions: | | | |
| N (4f) | 1/3 | 2/3 | 0.16836 |
| Mesh M-P | 16 × 16 × 12 | 308 pts | in IBZ |
| Energy | | -35.20070 eV | |

4 $\gamma N_2$:

| | | | |
|---|---|---|---|
| Space Group | $P4_2/mnm$ | $D_{4h}^{14}$ | #136 |
| Pearson Symbol | | tP4 | |
| $a$ , $b$ , $c$ | 3.70846Å | 3.70846Å | 4.97143Å |
| $\alpha$ , $\beta$ , $\gamma$ | 90° | 90° | 90° |
| Wyckoff Positions: | | | |
| N (4f) | 0.10517 | 0.10517 | 0 |
| Mesh M-P | 20 × 20 × 16 | 440 pts | in IBZ |
| Energy | | -35.26502 eV | |

5. $\varepsilon N_2$:

| | | | | |
|---|---|---|---|---|
| Space Group | | $R\bar{3}c$ | $D_{3d}^{6}$ | #167 |
| Pearson Symbol | | | hR48 | |
| $a$ , $b$ , $c$ | | 8.80174Å | 8.80174Å | 12.24907Å |
| $\alpha$ , $\beta$ , $\gamma$ | | 90° | 90° | 120° |
| Wyckoff Positions: | | | | |
| N | (12c) | 0 | 0 | 0.54502 |
| N | (36f) | 0.59839 | 0.87401 | 0.44383 |
| Mesh | M-P | $16 \times 16 \times 16$ | 408 pts | in IBZ |
| Energy | | | -141.00803 eV | |

6. $WN_4$ in $ReP_4$:
Within the LDA we found multiple solutions for $WN_4$ in the $ReP_4$ structure, that is, *Pbca* with all atoms on (8c) Wyckoff sites. We discuss two in the text. The first structure is close to that found by Aydin *et al.*[14]

| | | | | |
|---|---|---|---|---|
| Space Group | | *Pbca* | $D_{2h}^{15}$ | #61 |
| Pearson Symbol | | | oP40 | |
| $a$ , $b$ , $c$ | | 9.09251Å | 5.31379Å | 7.33060Å |
| $\alpha$ , $\beta$ , $\gamma$ | | 90° | 90° | 90° |
| Wyckoff Positions: | | | | |
| N | (8c) | 0.22549 | 0.67846 | 0.79285 |
| N | (8c) | 0.22037 | 0.78958 | 0.47263 |
| N | (8c) | 0.13816 | 0.30380 | 0.55204 |
| N | (8c) | 0.13922 | 0.17788 | 0.72096 |
| W | (8c) | 0.04474 | 0.66193 | 0.61748 |
| Mesh | Γ | $4 \times 6 \times 6$ | 48 pts | in IBZ |
| Energy | | | -384.91961 eV | |

However this structure has a much lower energy:

| | | | | |
|---|---|---|---|---|
| Space Group | | *Pbca* | $D_{2h}^{15}$ | #61 |
| Pearson Symbol | | | oP40 | |
| $a$ , $b$ , $c$ | | 9.66151Å | 6.27860Å | 7.53222Å |
| $\alpha$ , $\beta$ , $\gamma$ | | 90° | 90° | 90° |
| Wyckoff Positions: | | | | |
| N | (8c) | 0.23671 | 0.11094 | 0.77590 |
| N | (8c) | 0.74891 | 0.14662 | 0.56279 |
| N | (8c) | 0.00986 | 0.88265 | 0.66575 |
| N | (8c) | 0.97337 | 0.80102 | 0.80145 |
| W | (8c) | 0.13792 | 0.10610 | 0.56739 |
| Mesh | Γ | $4 \times 4 \times 6$ | 48 pts | in IBZ |
| Energy | | | -397.37447 eV | |

7. $WN_3$ in Molybdite ($MoO_3$) structure:

| | | | | |
|---|---|---|---|---|
| Space Group | | *Pnma* | $D_{2h}^{16}$ | #62 |
| Pearson Symbol | | | oP16 | |
| $a$ , $b$ , $c$ | | 18.23290Å | 4.00463Å | 2.86311Å |
| $\alpha$ , $\beta$ , $\gamma$ | | 90° | 90° | 90° |
| Wyckoff Positions: | | | | |
| N | (4c) | 0.53807 | 3/4 | 0.73906 |
| N | (4c) | 0.79737 | 3/4 | 0.20600 |
| N | (4c) | 0.59969 | 3/4 | 0.73406 |
| W | (4c) | 0.71097 | 3/4 | 0.70727 |
| Mesh | M-P | $6 \times 18 \times 24$ | 324 pts | in IBZ |
| Energy | | | -165.33052 eV | |

8. $WN_3$ in $P_3Tc$ structure:

| | | | | |
|---|---|---|---|---|
| Space Group | | *Pnma* | $D_{2h}^{16}$ | #62 |
| Pearson Symbol | | | oP16 | |
| $a$ , $b$ , $c$ | | 12.57592Å | 2.88205Å | 5.10810Å |
| $\alpha$ , $\beta$ , $\gamma$ | | 90° | 90° | 90° |
| Wyckoff Positions: | | | | |
| N | (4c) | 0.52322 | 3/4 | 0.21605 |
| N | (4c) | 0.93141 | 3/4 | 0.33998 |
| N | (4c) | 0.76902 | 3/4 | 0.76225 |
| W | (4c) | 0.66656 | 3/4 | 0.04584 |
| Mesh | M-P | $4 \times 16 \times 8$ | 64 pts | in IBZ |
| Energy | | | -165.89775 eV | |

9. $WN_2$ in lower symmetry structure of Wang *et al.*:[15]

| | | | | |
|---|---|---|---|---|
| Space Group | | $P\bar{6}m2$ | $D_{3h}^{1}$ | #187 |
| Pearson Symbol | | | hP3 | |
| $a$ , $b$ , $c$ | | 2.88726Å | 2.88726Å | 3.87688Å |
| $\alpha$ , $\beta$ , $\gamma$ | | 90° | 90° | 120° |
| Wyckoff Positions: | | | | |
| N | (2g) | 0 | 0 | 0.18044 |
| W | (1d) | 1/3 | 2/3 | 1/2 |
| Mesh | M-P | $16 \times 16 \times 12$ | 432 pts | in IBZ |
| Energy | | | -33.81916 eV | |

10. $WN_2$ in higher symmetry structure of Wang *et al.*:[15]

| Space Group | $P6_3/mmc$ | $D_{6h}^4$ | #194 |
|---|---|---|---|
| Pearson Symbol | | hP6 | |
| $a$ , $b$ , $c$ | 2.89316Å | 2.89316Å | 7.71367Å |
| $\alpha$ , $\beta$ , $\gamma$ | 90° | 90° | 120° |
| Wyckoff Positions: | | | |
| N (4e) | 0 | 0 | 0.08978 |
| W (2d) | 1/3 | 2/3 | 3/4 |
| Mesh M-P | $16 \times 16 \times 8$ | 288 pts | in IBZ |
| Energy | | -67.65958 eV | |

11. $WN_2$ in $CoSb_2$ structure:

| Space Group | $P2_1/c$ | $C_{2h}^5$ | #14 |
|---|---|---|---|
| Pearson Symbol | | mP12 | |
| $a$ , $b$ , $c$ | 4.85002Å | 4.89988Å | 5.12147Å |
| $\alpha$ , $\beta$ , $\gamma$ | 90° | 99.3565° | 90° |
| Wyckoff Positions: | | | |
| N (4e) | 0.43463 | 0.32878 | 0.16170 |
| N (4e) | 0.07383 | 0.73977 | 0.51917 |
| W (4e) | 0.21230 | 0.06261 | 0.28069 |
| Mesh M-P | $8 \times 8 \times 8$ | 128 pts | in IBZ |
| Energy | | -133.20703 eV | |

12. $WN_2$: constructed by removing 14 atoms from a 32 atom supercell of NaCl:

| Space Group | $Im\bar{3}m$ | $O_h^9$ | #229 |
|---|---|---|---|
| Pearson Symbol | | cI36 | |
| $a$ , $b$ , $c$ | 10.27372Å | 10.27372Å | 10.27372Å |
| $\alpha$ , $\beta$ , $\gamma$ | 90° | 90° | 90° |
| Wyckoff Positions: | | | |
| N (24h) | 0 | 0.35463 | 0.35463 |
| W (12d) | 0 | 1/4 | 1/2 |
| Mesh M-P | $10 \times 10 \times 10$ | 44 pts | in IBZ |
| Energy | | -195.48427 eV | |

13. $WN_2$ in $AuSn_2$ structure:

| Space Group | $Pbca$ | $D_{2h}^{15}$ | #61 |
|---|---|---|---|
| Pearson Symbol | | oP24 | |
| $a$ , $b$ , $c$ | 9.61612Å | 4.88812Å | 5.09072Å |
| $\alpha$ , $\beta$ , $\gamma$ | 90° | 90° | 90° |
| Wyckoff Positions: | | | |
| N (8c) | 0.96672 | 0.66613 | 0.67774 |
| N (8c) | 0.71228 | 0.74415 | 0.58230 |
| W (8c) | 0.64390 | 0.43772 | 0.82796 |
| Mesh Γ | $4 \times 8 \times 8$ | 75 pts | in IBZ |
| Energy | | -266.15819 eV | |

14. $WN_2$ in $Mo_2N$ structure:

| Space Group | $I4_1/amd$ | $D_{4h}^{19}$ | #141 |
|---|---|---|---|
| Pearson Symbol | | tI12 | |
| $a$ , $b$ , $c$ | 3.74217Å | 3.74217Å | 10.51044Å |
| $\alpha$ , $\beta$ , $\gamma$ | 90° | 90° | 90° |
| Wyckoff Positions: | | | |
| N (8e) | 0 | 3/4 | 0.92786 |
| W (4a) | 0 | 3/4 | 0.12500 |
| Mesh Γ | $12 \times 12 \times 20$ | 667 pts | in IBZ |
| Energy | | -65.64424 eV | |

15. $W_3N_4$ in $S_3U_4$ structure:[16]

| Space Group | $Pm\bar{3}m$ | $O_h^1$ | #221 |
|---|---|---|---|
| Pearson Symbol | | cP7 | |
| $a$ , $b$ , $c$ | 4.17013Å | 4.17013Å | 4.17013Å |
| $\alpha$ , $\beta$ , $\gamma$ | 90° | 90° | 90° |
| Wyckoff Positions: | | | |
| N (1a) | 0 | 0 | 0 |
| N (3c) | 1/2 | 0 | 1/2 |
| W (3d) | 0 | 1/2 | 0 |
| Mesh Γ | $22 \times 22 \times 22$ | 364 pts | in IBZ |
| Energy | | -80.34071 eV | |

16. $W_6N_7$: constructed by removing 3 atoms from a 16 atom supercell of NaCl:

| Space Group | $Fm\bar{3}m$ | $O_h^5$ | #225 |
|---|---|---|---|
| Pearson Symbol | | cF52 | |
| $a$ , $b$ , $c$ | 8.24485Å | 8.24485Å | 8.24485Å |
| $\alpha$ , $\beta$ , $\gamma$ | 90° | 90° | 90° |
| Wyckoff Positions: | | | |
| N (4b) | 1/2 | 1/2 | 1/2 |
| N (24d) | 1/2 | 1/4 | 1/4 |
| W (24e) | 0.23122 | 1/2 | 1/2 |
| Mesh Γ | $12 \times 12 \times 12$ | 72 pts | in IBZ |
| Energy | | -154.90404 eV | |

17. $W_{12}N_{13}$: constructed by removing 7 atoms from a 32 atom supercell of NaCl:

| | | | | |
|---|---|---|---|---|
| Space Group | | $Im\overline{3}m$ | $O_h^9$ | #229 |
| Pearson Symbol | | | cI50 | |
| $a$ , $b$ , $c$ | | 8.19323Å | 8.19323Å | 8.19323Å |
| $\alpha$ , $\beta$ , $\gamma$ | | 90° | 90° | 90° |
| Wyckoff Positions: | | | | |
| N | (2a) | 0 | 0 | 0 |
| N | (24h) | 0 | 0.25094 | 0.25094 |
| W | (12d) | 0 | 1/4 | 1/2 |
| W | (12e) | 0.26125 | 0 | 0 |
| Mesh | Γ | 12 × 12 × 12 | 72 pts | in IBZ |
| Energy | | -299.89601 eV | | |

18. WN: NbO structure – constructed by removing 2 atoms from an 8 atom supercell of NaCl. This is the ground state of WN.

| | | | | |
|---|---|---|---|---|
| Space Group | | $Pm\overline{3}m$ | $O_h^1$ | #221 |
| Pearson Symbol | | | cP6 | |
| $a$ , $b$ , $c$ | | 4.07801Å | 4.07801Å | 4.07801Å |
| $\alpha$ , $\beta$ , $\gamma$ | | 90° | 90° | 90° |
| Wyckoff Positions: | | | | |
| N | (3c) | 1/2 | 0 | 1/2 |
| W | (3d) | 0 | 1/2 | 0 |
| Mesh | Γ | 20 × 20 × 20 | 286 pts | in IBZ |
| Energy | | -72.81162 eV | | |

19. WN: constructed by removing 4 atoms from a 16 atom body-centered tetragonal supercell of NaCl:

| | | | | |
|---|---|---|---|---|
| Space Group | | $I4mm$ | $C_{4v}^9$ | #107 |
| Pearson Symbol | | | tI24 | |
| $a$ , $b$ , $c$ | | 4.10200Å | 4.10200Å | 16.26180Å |
| $\alpha$ , $\beta$ , $\gamma$ | | 90° | 90° | 90° |
| Wyckoff Positions: | | | | |
| N | (2a) | 0 | 0 | 0.49837 |
| N | (2a) | 0 | 0 | 0.25063 |
| N | (4b) | 1/2 | 0 | 0.12467 |
| N | (4b) | 0 | 1/2 | 0.37408 |
| W | (2a) | 0 | 0 | 0.88054 |
| W | (2a) | 0 | 0 | 0.62892 |
| W | (4b) | 0 | 1/2 | 0.49830 |
| W | (4b) | 0 | 1/2 | 0.24872 |
| Mesh | Γ | 12 × 12 × 8 | 234 pts | in IBZ |
| Energy | | -144.75026 eV | | |

20. WN: constructed by removing 2 atoms from an 8 atom body-centered tetragonal supercell of NaCl:

| | | | | |
|---|---|---|---|---|
| Space Group | | $I4mm$ | $C_{4v}^9$ | #107 |
| Pearson Symbol | | | tI12 | |
| $a$ , $b$ , $c$ | | 4.12998Å | 4.12998Å | 8.13034Å |
| $\alpha$ , $\beta$ , $\gamma$ | | 90° | 90° | 90° |
| Wyckoff Positions: | | | | |
| N | (2a) | 0 | 0 | 0.99315 |
| N | (4b) | 0 | 1/2 | 0.25443 |
| W | (2a) | 0 | 0 | 0.72998 |
| W | (4b) | 1/2 | 0 | 0.00901 |
| Mesh | Γ | 20 × 20 × 20 | 641 pts | in IBZ |
| Energy | | -72.13474 eV | | |

21. WN: Cubic Zincblende (B3) structure:

| | | | | |
|---|---|---|---|---|
| Space Group | | $F\overline{4}3m$ | $T_d^2$ | #216 |
| Pearson Symbol | | | cF8 | |
| $a$ , $b$ , $c$ | | 4.60727Å | 4.60727Å | 4.60727Å |
| $\alpha$ , $\beta$ , $\gamma$ | | 90° | 90° | 90° |
| Wyckoff Positions: | | | | |
| N | (4a) | 0 | 0 | 0 |
| W | (4d) | 3/4 | 3/4 | 3/4 |
| Mesh | Γ | 24 × 24 × 24 | 413 pts | in IBZ |
| Energy | | -23.06926 eV | | |

22. WN: NaCl (B1) structure:

| | | | | |
|---|---|---|---|---|
| Space Group | | $Fm\overline{3}m$ | $O_h^5$ | #225 |
| Pearson Symbol | | | cF8 | |
| $a$ , $b$ , $c$ | | 4.30140Å | 4.30140Å | 4.30140Å |
| $\alpha$ , $\beta$ , $\gamma$ | | 90° | 90° | 90° |
| Wyckoff Positions: | | | | |
| N | (4a) | 0 | 0 | 0 |
| W | (4b) | 1/2 | 1/2 | 1/2 |
| Mesh | Γ | 24 × 24 × 24 | 413 pts | in IBZ |
| Energy | | -22.99192 eV | | |

23. $W_{13}N_{12}$: complementary structure to $W_{12}N_{13}$

| | | | | |
|---|---|---|---|---|
| Space Group | | $Im\bar{3}m$ | $O_h^9$ | #229 |
| Pearson Symbol | | | cI50 | |
| $a$ , $b$ , $c$ | | 8.22119Å | 8.22119Å | 8.22119Å |
| $\alpha$ , $\beta$ , $\gamma$ | | 90° | 90° | 90° |
| Wyckoff Positions: | | | | |
| N | (12d) | 0 | 1/4 | 1/2 |
| N | (12e) | 0.26197 | 0 | 0 |
| W | (2a) | 0 | 0 | 0 |
| W | (24h) | 0 | 0.25287 | 0.25287 |
| Mesh | Γ | 12 × 12 × 12 | 72 pts | in IBZ |
| Energy | | | -305.03302 eV | |

24. $W_4N_3$ in $S_3U_4$ structure:

| | | | | |
|---|---|---|---|---|
| Space Group | | $Pm\bar{3}m$ | $O_h^1$ | #221 |
| Pearson Symbol | | | cP7 | |
| $a$ , $b$ , $c$ | | 4.23177Å | 4.23177Å | 4.23177Å |
| $\alpha$ , $\beta$ , $\gamma$ | | 90° | 90° | 90° |
| Wyckoff Positions: | | | | |
| N | (3d) | 0 | 1/2 | 0 |
| W | (1a) | 0 | 0 | 0 |
| W | (3c) | 1/2 | 0 | 1/2 |
| Mesh | Γ | 22 × 22 × 22 | 364 pts | in IBZ |
| Energy | | | -84.32493 eV | |

25. $W_3N_2$: This is the hexagonal $\delta_H^I$ phase described by Khitrova and Pinkser,[17] however we assume that all the (4f) sites are fully occupied.

| | | | | |
|---|---|---|---|---|
| Space Group | | $P6_3/mmc$ | $D_{6h}^4$ | #194 |
| Pearson Symbol | | | hP10 | |
| $a$ , $b$ , $c$ | | 2.85564Å | 2.85564Å | 15.69825Å |
| $\alpha$ , $\beta$ , $\gamma$ | | 90° | 90° | 120° |
| Wyckoff Positions: | | | | |
| N | (4f) | 2/3 | 1/3 | 0.16195 |
| W | (2c) | 2/3 | 1/3 | 3/4 |
| W | (4f) | 2/3 | 1/3 | 0.93012 |
| Mesh | Γ | 18 × 18 × 12 | 259 pts | in IBZ |
| Energy | | | -124.87489 eV | |

26. $W_2N$ in $MoS_2$ (C7) structure:

| | | | | |
|---|---|---|---|---|
| Space Group | | $P6_3/mmc$ | $D_{6h}^4$ | #194 |
| Pearson Symbol | | | hP6 | |
| $a$ , $b$ , $c$ | | 2.83724Å | 2.83724Å | 10.21272Å |
| $\alpha$ , $\beta$ , $\gamma$ | | 90° | 90° | 120° |
| Wyckoff Positions: | | | | |
| N | (2c) | 1/3 | 2/3 | 1/4 |
| W | (4f) | 1/3 | 2/3 | 0.88829 |
| Mesh | Γ | 16 × 16 × 4 | 90 pts | in IBZ |
| Energy | | | -76.54735 eV | |

27. $W_2N$ in $Mo_2N$ structure:

| | | | | |
|---|---|---|---|---|
| Space Group | | $I4_1/amd$ | $D_{4h}^{19}$ | #141 |
| Pearson Symbol | | | tI12 | |
| $a$ , $b$ , $c$ | | 4.23644Å | 4.23644Å | 7.89086Å |
| $\alpha$ , $\beta$ , $\gamma$ | | 90° | 90° | 90° |
| Wyckoff Positions: | | | | |
| N | (4b) | 1/2 | 1/4 | 0.12500 |
| W | (8e) | 0 | 3/4 | 0.89014 |
| Mesh | Γ | 10 × 10 × 18 | 474 pts | in IBZ |
| Energy | | | -75.88729 eV | |

28. $W_2N$: Complementary structure to cubic $WN_2$ structure with space group $Im\bar{3}m$

| | | | | |
|---|---|---|---|---|
| Space Group | | $Im\bar{3}m$ | $O_h^9$ | #229 |
| Pearson Symbol | | | cI36 | |
| $a$ , $b$ , $c$ | | 7.94613Å | 7.94613Å | 7.94613Å |
| $\alpha$ , $\beta$ , $\gamma$ | | 90° | 90° | 90° |
| Wyckoff Positions: | | | | |
| N | (12d) | 0 | 1/4 | 1/2 |
| W | (24h) | 0 | 0.24609 | 0.24609 |
| Mesh | Γ | 12 × 12 × 12 | 72 pts | in IBZ |
| Energy | | | -218.29059 eV | |

29. $W_3N$: $MoO_3$ structure. Ordinarily this structure is in space group $Pnma$, but we found that it relaxes to a higher symmetry structure independent of the choice of density functional.

| | | | | |
|---|---|---|---|---|
| Space Group | | $Cmcm$ | $D_{2h}^{17}$ | #63 |
| Pearson Symbol | | | oC16 | |
| $a$ , $b$ , $c$ | | 4.17491Å | 11.85749Å | 4.15521Å |
| $\alpha$ , $\beta$ , $\gamma$ | | 90° | 90° | 90° |
| Wyckoff Positions: | | | | |
| N | (4c) | 1/2 | 0.42207 | 3/4 |
| W | (4c) | 1/2 | 0.60101 | 3/4 |
| W | (4c) | 1/2 | 0.91447 | 3/4 |
| W | (4c) | 1/2 | 0.24463 | 3/4 |
| Mesh | Γ | $12 \times 12 \times 16$ | 397 pts | in IBZ |
| Energy | | | -104.09407 eV | |

30. $W_3N$: $P_3Tc$ structure:

| | | | | |
|---|---|---|---|---|
| Space Group | | $Pnma$ | $D_{2h}^{16}$ | #62 |
| Pearson Symbol | | | oP16 | |
| $a$ , $b$ , $c$ | | 15.70481Å | 2.91338Å | 4.58860Å |
| $\alpha$ , $\beta$ , $\gamma$ | | 90° | 90° | 90° |
| Wyckoff Positions: | | | | |
| N | (4c) | 0.66423 | 3/4 | 0.98928 |
| W | (4c) | 0.55168 | 3/4 | 0.74009 |
| W | (4c) | 0.88491 | 3/4 | 0.76705 |
| W | (4c) | 0.77673 | 3/4 | 0.23188 |
| Mesh | Γ | $4 \times 14 \times 10$ | 144 pts | in IBZ |
| Energy | | | -204.92082 eV | |

31. $W_4N$: $ReP_4$ structure:

| | | | | |
|---|---|---|---|---|
| Space Group | | $Pbca$ | $D_{2h}^{15}$ | #61 |
| Pearson Symbol | | | oP40 | |
| $a$ , $b$ , $c$ | | 11.56201Å | 5.00816Å | 9.29737Å |
| $\alpha$ , $\beta$ , $\gamma$ | | 90° | 90° | 90° |
| Wyckoff Positions: | | | | |
| N | (8c) | 0.06171 | 0.42239 | 0.37980 |
| W | (8c) | 0.19046 | 0.60451 | 0.25656 |
| W | (8c) | 0.18778 | 0.24660 | 0.50515 |
| W | (8c) | 0.06899 | 0.77376 | 0.50302 |
| W | (8c) | 0.06849 | 0.08909 | 0.24816 |
| Mesh | Γ | $4 \times 8 \times 4$ | 45 pts | in IBZ |
| Energy | | | -525.67476 eV | |

32. W: BCC (A2) ground state:

| | | | | |
|---|---|---|---|---|
| Space Group | | $Im\bar{3}m$ | $O_h^9$ | #229 |
| Pearson Symbol | | | cI2 | |
| $a$ , $b$ , $c$ | | 3.14264Å | 3.14264Å | 3.14264Å |
| $\alpha$ , $\beta$ , $\gamma$ | | 90° | 90° | 90° |
| Wyckoff Positions: | | | | |
| W | (2a) | 0 | 0 | 0 |
| Mesh | Γ | $32 \times 32 \times 32$ | 897 pts | in IBZ |
| Energy | | | -14.04786 eV | |

33. W: $\beta$-W (A15):

| | | | | |
|---|---|---|---|---|
| Space Group | | $Pm\bar{3}n$ | $O_h^3$ | #223 |
| Pearson Symbol | | | cP8 | |
| $a$ , $b$ , $c$ | | 5.01509Å | 5.01509Å | 5.01509Å |
| $\alpha$ , $\beta$ , $\gamma$ | | 90° | 90° | 90° |
| Wyckoff Positions: | | | | |
| W | (2a) | 1/2 | 1/2 | 1/2 |
| W | (6d) | 0 | 1/4 | 1/2 |
| Mesh | Γ | $16 \times 16 \times 16$ | 165 pts | in IBZ |
| Energy | | | -13.55857 eV | |

34. W: FCC (A1):

| | | | | |
|---|---|---|---|---|
| Space Group | | $Fm\bar{3}m$ | $O_h^5$ | #225 |
| Pearson Symbol | | | cF4 | |
| $a$ , $b$ , $c$ | | 3.98139Å | 3.98139Å | 3.98139Å |
| $\alpha$ , $\beta$ , $\gamma$ | | 90° | 90° | 90° |
| Wyckoff Positions: | | | | |
| W | (4a) | 0 | 0 | 0 |
| Mesh | Γ | $32 \times 32 \times 32$ | 897 pts | in IBZ |
| Energy | | | -111.59262 eV | |

## III. PERDEW-BURKE-ERNZERHOF (PBE)[12] GENERALIZED GRADIENT APPROXIMATION

For comments on the individual phases see Sec. II.

1. $\alpha N_2$: High symmetry state:

| | | | | |
|---|---|---|---|---|
| Space Group | | $Pa\bar{3}$ | $T_h^6$ | #205 |
| Pearson Symbol | | | cP8 | |
| $a$ , $b$ , $c$ | | 6.18740Å | 6.18740Å | 6.18740Å |
| $\alpha$ , $\beta$ , $\gamma$ | | 90° | 90° | 90° |
| Wyckoff Positions: | | | | |
| N | (8c) | 0.55192 | 0.44808 | 0.94808 |
| Mesh | Γ | $16 \times 16 \times 16$ | 249 pts | in IBZ |
| Energy | | | -66.65799 eV | |

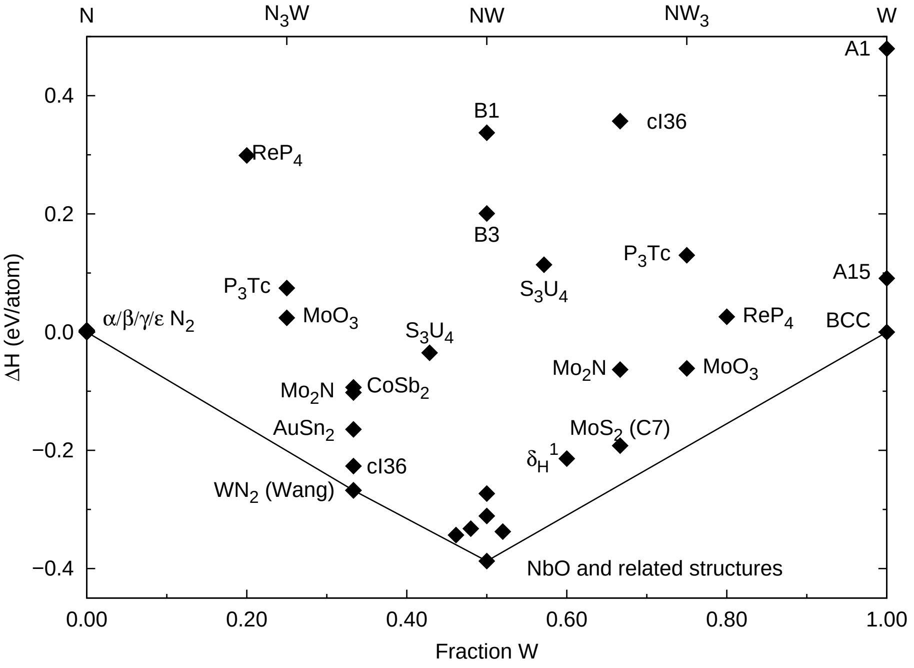


FIG. 2. Enthalpy per atom for $N_{1-x}W_x$ using the Perdew-Burk-Ernzerhof Approximation

2. $\alpha N_2$: Low symmetry state:

| Space Group | | $P2_13$ | $T^4$ | #198 |
|---|---|---|---|---|
| Pearson Symbol | | | cP8 | |
| $a$ , $b$ , $c$ | | 6.18848Å | 6.18848Å | 6.18848Å |
| $\alpha$ , $\beta$ , $\gamma$ | | 90° | 90° | 90° |
| Wyckoff Positions: | | | | |
| N | (4a) | 0.30285 | 0.19715 | 0.80285 |
| N | (4a) | 0.19903 | 0.30097 | 0.69903 |
| Mesh | Γ | 16 × 16 × 16 | 249 pts | in IBZ |
| Energy | | | -66.65801 eV | |

3. $\beta N_2$:

| Space Group | | $P6_3/mmc$ | $D^4_{6h}$ | #194 |
|---|---|---|---|---|
| Pearson Symbol | | | hP4 | |
| $a$ , $b$ , $c$ | | 5.32369Å | 5.32369Å | 5.99005Å |
| $\alpha$ , $\beta$ , $\gamma$ | | 90° | 90° | 120° |
| Wyckoff Positions: | | | | |
| N | (4f) | 1/3 | 2/3 | 0.15710 |
| Mesh | Γ | 20 × 20 × 20 | 484 pts | in IBZ |
| Energy | | | -33.31655 eV | |

4. $\gamma N_2$:

| Space Group | | $P4_2/mnm$ | $D^{14}_{4h}$ | #136 |
|---|---|---|---|---|
| Pearson Symbol | | | tP4 | |
| $a$ , $b$ , $c$ | | 4.42366Å | 4.42366Å | 6.00037Å |
| $\alpha$ , $\beta$ , $\gamma$ | | 90° | 90° | 90° |
| Wyckoff Positions: | | | | |
| N | (4f) | 0.58895 | 0.58895 | 0 |
| Mesh | Γ | 20 × 20 × 15 | 528 pts | in IBZ |
| Energy | | | -33.32787 | |

5. $\varepsilon N_2$:

| Space Group | | $R\bar{3}c$ | $D^6_{3d}$ | #167 |
|---|---|---|---|---|
| Pearson Symbol | | | hR48 | |
| $a$ , $b$ , $c$ | | 10.79199Å | 10.79199Å | 14.22027Å |
| $\alpha$ , $\beta$ , $\gamma$ | | 90° | 90° | 120° |
| Wyckoff Positions: | | | | |
| N | (12c) | 0 | 0 | 0.53913 |
| N | (36f) | 0.59936 | 0.88419 | 0.43936 |
| Mesh | Γ | 12 × 12 × 12 | pts | in IBZ |
| Energy | | | -133.29051 eV | |

6. $WN_4$ $ReP_4$: Although multiple solutions for the $ReP_4$ structure undoubtably exist, here we only show the lowest energy state we have found so far. We started this calculation with the structure proposed by Aydin *et al.*,[14] but it quickly relaxed to a structure similar to the one shown below.

| | | | | |
|---|---|---|---|---|
| Space Group | | $Pbca$ | $D_{2h}^{15}$ | #61 |
| Pearson Symbol | | | oP40 | |
| $a$ , $b$ , $c$ | | 13.27276Å | 4.92710Å | 8.40170Å |
| $\alpha$ , $\beta$ , $\gamma$ | | 90° | 90° | 90° |
| Wyckoff Positions: | | | | |
| N | (8c) | 0.15396 | 0.66482 | 0.79640 |
| N | (8c) | 0.15135 | 0.76724 | 0.43052 |
| N | (8c) | 0.03993 | 0.25582 | 0.58381 |
| N | (8c) | 0.03215 | 0.06852 | 0.69119 |
| W | (8c) | 0.05629 | 0.66194 | 0.60742 |
| Mesh | Γ | $4 \times 6 \times 6$ | 48 pts | in IBZ |
| Energy | | | -358.37447 eV | |

7. $WN_3$ in Molybdite ($MoO_3$) structure:

| | | | | |
|---|---|---|---|---|
| Space Group | | $Pnma$ | $D_{2h}^{16}$ | #62 |
| Pearson Symbol | | | oP16 | |
| $a$ , $b$ , $c$ | | 21.19384Å | 4.05147Å | 2.92603Å |
| $\alpha$ , $\beta$ , $\gamma$ | | 90° | 90° | 90° |
| Wyckoff Positions: | | | | |
| N | (4c) | 0.56477 | 3/4 | 0.21841 |
| N | (4c) | 0.79123 | 3/4 | 0.70611 |
| N | (4c) | 0.61815 | 3/4 | 0.21652 |
| W | (4c) | 0.71612 | 3/4 | 0.20661 |
| Mesh | Γ | $5 \times 21 \times 29$ | 495 pts | in IBZ |
| Energy | | | -151.44786 eV | |

8. $WN_3$ in $P_3Tc$ structure:

| | | | | |
|---|---|---|---|---|
| Space Group | | $Pnma$ | $D_{2h}^{16}$ | #62 |
| Pearson Symbol | | | oP16 | |
| $a$ , $b$ , $c$ | | 12.65081Å | 2.93872Å | 5.28463Å |
| $\alpha$ , $\beta$ , $\gamma$ | | 90° | 90° | 90° |
| Wyckoff Positions: | | | | |
| N | (4c) | 0.02675 | 3/4 | 0.20824 |
| N | (4c) | 0.43410 | 3/4 | 0.33688 |
| N | (4c) | 0.26605 | 3/4 | 0.73991 |
| W | (4c) | 0.16889 | 3/4 | 0.02906 |
| Mesh | Γ | $8 \times 24 \times 16$ | 585 pts | in IBZ |
| Energy | | | -150.64464 eV | |

9. $WN_2$ in lower symmetry structure of Wang *et al.*[15]:

| | | | | |
|---|---|---|---|---|
| Space Group | | $P\bar{6}m2$ | $D_{3h}^{1}$ | #187 |
| Pearson Symbol | | | hP3 | |
| $a$ , $b$ , $c$ | | 2.93342Å | 2.93342Å | 3.91819Å |
| $\alpha$ , $\beta$ , $\gamma$ | | 90° | 90° | 120° |
| Wyckoff Positions: | | | | |
| N | (2g) | 0 | 0 | 0.18136 |
| W | (1d) | 1/3 | 2/3 | 1/2 |
| Mesh | Γ | $33 \times 33 \times 22$ | 1296 pts | in IBZ |
| Energy | | | -30.42911 eV | |

10. $WN_2$ in higher symmetry structure of[15] Wang et al.:

| | | | | |
|---|---|---|---|---|
| Space Group | | $P6_3/mmc$ | $D_{6h}^{4}$ | #194 |
| Pearson Symbol | | | hP6 | |
| $a$ , $b$ , $c$ | | 2.93922Å | 2.93922Å | 7.79617Å |
| $\alpha$ , $\beta$ , $\gamma$ | | 90° | 90° | 120° |
| Wyckoff Positions: | | | | |
| N | (4e) | 0 | 0 | 0.09016 |
| W | (2d) | 1/3 | 2/3 | 3/4 |
| Mesh | Γ | $33 \times 33 \times 11$ | 684 pts | in IBZ |
| Energy | | | -60.85789 eV | |

11. $WN_2$ in $CoSb_2$ structure:

| | | | | |
|---|---|---|---|---|
| Space Group | | $P2_1/c$ | $C_{2h}^{5}$ | #14 |
| Pearson Symbol | | | mP12 | |
| $a$ , $b$ , $c$ | | 4.85002Å | 4.89988Å | 5.12147Å |
| $\alpha$ , $\beta$ , $\gamma$ | | 90° | 99.3565° | 90° |
| Wyckoff Positions: | | | | |
| N | (4e) | 0.43463 | 0.32878 | 0.16170 |
| N | (4e) | 0.07383 | 0.73977 | 0.51917 |
| W | (4e) | 0.21230 | 0.06261 | 0.28069 |
| Mesh | M-P | $8 \times 8 \times 8$ | 128 pts | in IBZ |
| Energy | | | -133.20703 eV | |

12. $WN_2$: constructed by removing 14 atoms from a 32 atom supercell of NaCl:

| | | | | |
|---|---|---|---|---|
| Space Group | | $Im\bar{3}m$ | $O_h^9$ | #229 |
| Pearson Symbol | | | cI36 | |
| $a$ , $b$ , $c$ | | 10.38300Å | 10.38300Å | 10.38300Å |
| $\alpha$ , $\beta$ , $\gamma$ | | 90° | 90° | 90° |
| Wyckoff Positions: | | | | |
| N | (24h) | 0 | 0.35454 | 0.35454 |
| W | (12d) | 0 | 1/4 | 1/2 |
| Mesh | M-P | $12 \times 12 \times 12$ | 72 pts | in IBZ |
| Energy | | | -181.83350 eV | |

13. $WN_2$ in $AuSn_2$ structure:

| | | | |
|---|---|---|---|
| Space Group | *Pbca* | $D_{2h}^{15}$ | #61 |
| Pearson Symbol | | oP24 | |
| $a$ , $b$ , $c$ | 9.77240Å | 4.95123Å | 5.16705Å |
| $\alpha$ , $\beta$ , $\gamma$ | 90° | 90° | 90° |
| Wyckoff Positions: | | | |
| N (8c) | 0.96657 | 0.66855 | 0.67720 |
| N (8c) | 0.71325 | 0.74383 | 0.58067 |
| W (8c) | 0.64349 | 0.43740 | 0.82628 |
| Mesh Γ | 9 × 17 × 17 | 405 pts | in IBZ |
| Energy | | -240.95494 eV | |

14. $WN_2$ in $Mo_2N$ structure:

| | | | |
|---|---|---|---|
| Space Group | $I4_1/amd$ | $D_{4h}^{19}$ | #141 |
| Pearson Symbol | | tI12 | |
| $a$ , $b$ , $c$ | 3.79214Å | 3.79214Å | 10.63734Å |
| $\alpha$ , $\beta$ , $\gamma$ | 90° | 90° | 90° |
| Wyckoff Positions: | | | |
| N (8e) | 1/2 | 1/4 | 0.92784 |
| W (4b) | 1/2 | 1/4 | 0.12500 |
| Mesh Γ | 12 × 12 × 20 | 667 pts | in IBZ |
| Energy | | -59.86539 eV | |

15. $W_3N_4$ in $S_3U_4$ structure:

| | | | |
|---|---|---|---|
| Space Group | $Pm\overline{3}m$ | $O_h^1$ | #221 |
| Pearson Symbol | | cP7 | |
| $a$ , $b$ , $c$ | 4.22769Å | 4.22769Å | 4.22769Å |
| $\alpha$ , $\beta$ , $\gamma$ | 90° | 90° | 90° |
| Wyckoff Positions: | | | |
| N (1a) | 0 | 0 | 0 |
| N (3c) | 1/2 | 0 | 1/2 |
| W (3d) | 0 | 1/2 | 0 |
| Mesh Γ | 22 × 22 × 22 | 364 pts | in IBZ |
| Energy | | -72.45771 eV | |

16. $W_6N_7$: constructed by removing 3 atoms from a 16 atom supercell of NaCl:

| | | | |
|---|---|---|---|
| Space Group | $Fm\overline{3}m$ | $O_h^5$ | #225 |
| Pearson Symbol | | cF52 | |
| $a$ , $b$ , $c$ | 8.35636Å | 8.35636Å | 8.35636Å |
| $\alpha$ , $\beta$ , $\gamma$ | 90° | 90° | 90° |
| Wyckoff Positions: | | | |
| N (4b) | 1/2 | 1/2 | 1/2 |
| N (24d) | 1/4 | 1/4 | 1/2 |
| W (24e) | 1/2 | 1/2 | 0.23068 |
| Mesh Γ | 18 × 18 × 18 | 195 pts | in IBZ |
| Energy | | -140.55665 eV | |

17. $W_{12}N_{13}$: constructed by removing 7 atoms from a 32 atom supercell of NaCl:

| | | | |
|---|---|---|---|
| Space Group | $Im\overline{3}m$ | $O_h^9$ | #229 |
| Pearson Symbol | | cI50 | |
| $a$ , $b$ , $c$ | 8.30255Å | 8.30255Å | 8.30255Å |
| $\alpha$ , $\beta$ , $\gamma$ | 90° | 90° | 90° |
| Wyckoff Positions: | | | |
| N (2a) | 0 | 0 | 0 |
| N (24h) | 0 | 0.25090 | 0.25090 |
| W (12d) | 0 | 1/4 | 1/2 |
| W (12e) | 0.26217 | 0 | 0 |
| Mesh Γ | 15 × 15 × 15 | 120 pts | in IBZ |
| Energy | | -272.16721 eV | |

18. WN: NbO structure

| | | | |
|---|---|---|---|
| Space Group | $Pm\overline{3}m$ | $O_h^1$ | #221 |
| Pearson Symbol | | cP6 | |
| $a$ , $b$ , $c$ | 4.13144Å | 4.13144Å | 4.13144Å |
| $\alpha$ , $\beta$ , $\gamma$ | 90° | 90° | 90° |
| Wyckoff Positions: | | | |
| N (3c) | 1/2 | 0 | 1/2 |
| W (3d) | 0 | 1/2 | 0 |
| Mesh Γ | 20 × 20 × 20 | 286 pts | in IBZ |
| Energy | | -66.20467 eV | |

19. WN: constructed by removing 4 atoms from a 16 atom body-centered tetragonal supercell of NaCl:

| | | | |
|---|---|---|---|
| Space Group | $I4mm$ | $C_{4v}^9$ | #107 |
| Pearson Symbol | | tI24 | |
| $a$ , $b$ , $c$ | 4.15925Å | 4.15925Å | 16.47511Å |
| $\alpha$ , $\beta$ , $\gamma$ | 90° | 90° | 90° |
| Wyckoff Positions: | | | |
| N (2a) | 0 | 0 | 0.49951 |
| N (2a) | 0 | 0 | 0.25072 |
| N (4b) | 0 | 1/2 | 0.12407 |
| N (4b) | 1/2 | 0 | 0.37401 |
| W (2a) | 0 | 0 | 0.88116 |
| W (2a) | 0 | 0 | 0.63043 |
| W (4b) | 1/2 | 0 | 0.49776 |
| W (4b) | 1/2 | 0 | 0.24825 |
| Mesh Γ | 16 × 16 × 16 | 349 pts | in IBZ |
| Energy | | -131.49430 eV | |

20. WN: constructed by removing 2 atoms from an 8 atom body-centered tetragonal supercell of NaCl:

| Space Group | | $I4mm$ | $C_{4v}^{9}$ | #107 |
|---|---|---|---|---|
| Pearson Symbol | | | tI12 | |
| $a$ , $b$ , $c$ | | 4.18771Å | 4.18771Å | 8.24079Å |
| $\alpha$ , $\beta$ , $\gamma$ | | 90° | 90° | 90° |
| Wyckoff Positions: | | | | |
| N | (2a) | 0 | 0 | 0.99220 |
| N | (4b) | 0 | 1/2 | 0.25473 |
| W | (2a) | 0 | 0 | 0.72855 |
| W | (4b) | 1/2 | 0 | 0.00989 |
| Mesh | Γ | 20 × 20 × 20 | 641 pts | in IBZ |
| Energy | | | -65.51907 eV | |

21. WN: Cubic Zincblende (B3) structure:

| Space Group | | $F\bar{4}3m$ | $T_{d}^{2}$ | #216 |
|---|---|---|---|---|
| Pearson Symbol | | | cF8 | |
| $a$ , $b$ , $c$ | | 4.67252Å | 4.67252Å | 4.67252Å |
| $\alpha$ , $\beta$ , $\gamma$ | | 90° | 90° | 90° |
| Wyckoff Positions: | | | | |
| N | (4a) | 0 | 0 | 0 |
| W | (4d) | 3/4 | 3/4 | 3/4 |
| Mesh | Γ | 34 × 34 × 34 | 1059 pts | in IBZ |
| Energy | | | -20.89222 eV | |

22. WN: NaCl (B1) structure:

| Space Group | | $Fm\bar{3}m$ | $O_{h}^{5}$ | #225 |
|---|---|---|---|---|
| Pearson Symbol | | | cF8 | |
| $a$ , $b$ , $c$ | | 4.36588Å | 4.36588Å | 4.36588Å |
| $\alpha$ , $\beta$ , $\gamma$ | | 90° | 90° | 90° |
| Wyckoff Positions: | | | | |
| N | (4a) | 0 | 0 | 0 |
| W | (4b) | 1/2 | 1/2 | 1/2 |
| Mesh | Γ | 34 × 34 × 34 | 1059 pts | in IBZ |
| Energy | | | -20.61895 eV | |

23. $W_{13}N_{12}$: complementary structure to $W_{12}N_{13}$.

| Space Group | | $Im\bar{3}m$ | $O_{h}^{9}$ | #229 |
|---|---|---|---|---|
| Pearson Symbol | | | cI50 | |
| $a$ , $b$ , $c$ | | 8.33189Å | 8.33189Å | 8.33189Å |
| $\alpha$ , $\beta$ , $\gamma$ | | 90° | 90° | 90° |
| Wyckoff Positions: | | | | |
| N | (12d) | 0 | 1/4 | 1/2 |
| N | (12e) | 0.26195 | 0 | 0 |
| W | (2a) | 0 | 0 | 0 |
| W | (24h) | 0 | 0.25297 | 0.25297 |
| Mesh | Γ | 15 × 15 × 15 | 120 pts | in IBZ |
| Energy | | | -276.92205 eV | |

24. $W_4N_3$ in $S_3U_4$ structure:

| Space Group | | $Pm\bar{3}m$ | $O_{h}^{1}$ | #221 |
|---|---|---|---|---|
| Pearson Symbol | | | cP7 | |
| $a$ , $b$ , $c$ | | 4.29301Å | 4.29301Å | 4.29301Å |
| $\alpha$ , $\beta$ , $\gamma$ | | 90° | 90° | 90° |
| Wyckoff Positions: | | | | |
| N | (3d) | 0 | 1/2 | 0 |
| W | (1a) | 0 | 0 | 0 |
| W | (3c) | 1/2 | 0 | 1/2 |
| Mesh | Γ | 22 × 22 × 22 | 364 pts | in IBZ |
| Energy | | | -76.04338 eV | |

25. $WN_{23}$: hexagonal $\delta_{H}^{I}$ phase:

| Space Group | | $P6_3/mmc$ | $D_{6h}^{4}$ | #194 |
|---|---|---|---|---|
| Pearson Symbol | | | hP10 | |
| $a$ , $b$ , $c$ | | 2.89592Å | 2.89592Å | 15.92141Å |
| $\alpha$ , $\beta$ , $\gamma$ | | 90° | 90° | 120° |
| Wyckoff Positions: | | | | |
| N | (4f) | 2/3 | 1/3 | 0.16237 |
| W | (2c) | 2/3 | 1/3 | 3/4 |
| W | (4f) | 2/3 | 1/3 | 0.93052 |
| Mesh | Γ | 34 × 34 × 6 | 456 pts | in IBZ |
| Energy | | | -113.23773 eV | |

26. $W_2N$ in $MoS_2$ (C7) structure: :

| Space Group | | $P6_3/mmc$ | $D_{6h}^{4}$ | #194 |
|---|---|---|---|---|
| Pearson Symbol | | | hP6 | |
| $a$ , $b$ , $c$ | | 2.87530Å | 2.87530Å | 10.37175Å |
| $\alpha$ , $\beta$ , $\gamma$ | | 90° | 90° | 120° |
| Wyckoff Positions: | | | | |
| N | (2d) | 2/3 | 1/3 | 1/4 |
| W | (4f) | 2/3 | 1/3 | 0.61160 |
| Mesh | Γ | 34 × 34 × 9 | 570 pts | in IBZ |
| Energy | | | -69.66272 eV | |

27. $W_2N$ in $Mo_2N$ structure:

| | | | | |
|---|---|---|---|---|
| Space Group | | $I4_1/amd$ | $D_{4h}^{19}$ | #141 |
| Pearson Symbol | | | tI12 | |
| $a$ , $b$ , $c$ | | 4.30206Å | 4.30206Å | 7.98537Å |
| $\alpha$ , $\beta$ , $\gamma$ | | 90° | 90° | 90° |
| Wyckoff Positions: | | | | |
| N | (4a) | 0 | 3/4 | 0.12500 |
| W | (8e) | 1/2 | 1/4 | 0.89096 |
| Mesh | Γ | 10 × 10 × 18 | 474 pts | in IBZ |
| Energy | | | -68.88987 eV | |

28. $W_2N$: Complementary structure to cubic $WN_2$ structure with space group $Im\overline{3}m$:

| | | | | |
|---|---|---|---|---|
| Space Group | | $Im\overline{3}m$ | $O_h^9$ | #229 |
| Pearson Symbol | | | cI36 | |
| $a$ , $b$ , $c$ | | 8.06722Å | 8.06722Å | 8.06722Å |
| $\alpha$ , $\beta$ , $\gamma$ | | 90° | 90° | 90° |
| Wyckoff Positions: | | | | |
| N | (12d) | 0 | 1/4 | 1/2 |
| W | (24h) | 0 | 0.24668 | 0.24668 |
| Mesh | Γ | 12 × 12 × 12 | 72 pts | in IBZ |
| Energy | | | -199.104831 eV | |

29. $W_3N$: $MoO_3$ structure. Again, it relaxes to a higher symmetry structure:

| | | | | |
|---|---|---|---|---|
| Space Group | | $Cmcm$ | $D_{2h}^{17}$ | #63 |
| Pearson Symbol | | | oC16 | |
| $a$ , $b$ , $c$ | | 4.23377Å | 12.03819Å | 4.21354Å |
| $\alpha$ , $\beta$ , $\gamma$ | | 90° | 90° | 90° |
| Wyckoff Positions: | | | | |
| N | (4c) | 1/2 | 0.42260 | 3/4 |
| W | (4c) | 1/2 | 0.60188 | 3/4 |
| W | (4c) | 1/2 | 0.91454 | 3/4 |
| W | (4c) | 1/2 | 0.24481 | 3/4 |
| Mesh | Γ | 12 × 12 × 16 | 387 pts | in IBZ |
| Energy | | | -94.92274 eV | |

30. $W_3N$: $P_3Tc$ structure:

| | | | | |
|---|---|---|---|---|
| Space Group | | $Pnma$ | $D_{2h}^{16}$ | #62 |
| Pearson Symbol | | | oP16 | |
| $a$ , $b$ , $c$ | | 15.96981Å | 2.93765Å | 4.66695Å |
| $\alpha$ , $\beta$ , $\gamma$ | | 90° | 90° | 90° |
| Wyckoff Positions: | | | | |
| N | (4c) | 0.83591 | 3/4 | 0.51206 |
| W | (4c) | 0.94810 | 3/4 | 0.76009 |
| W | (4c) | 0.61418 | 3/4 | 0.73154 |
| W | (4c) | 0.72454 | 3/4 | 0.26864 |
| Mesh | Γ | 6 × 29 × 18 | 484 pts | in IBZ |
| Energy | | | -186.78387 eV | |

31. $W_4N$: $ReP_4$ structure:

| | | | | |
|---|---|---|---|---|
| Space Group | | $Pbca$ | $D_{2h}^{15}$ | #61 |
| Pearson Symbol | | | oP40 | |
| $a$ , $b$ , $c$ | | 9.43000Å | 11.73041Å | 5.08234Å |
| $\alpha$ , $\beta$ , $\gamma$ | | 90° | 90° | 90° |
| Wyckoff Positions: | | | | |
| N | (8c) | 0.37955 | 0.56152 | 0.92274 |
| W | (8c) | 0.25672 | 0.69035 | 0.10609 |
| W | (8c) | 0.50484 | 0.68735 | 0.74693 |
| W | (8c) | 0.50337 | 0.56922 | 0.27410 |
| W | (8c) | 0.24796 | 0.56898 | 0.58966 |
| Mesh | Γ | 9 × 8 × 17 | 225 pts | in IBZ |
| Energy | | | -480.38270 eV | |

32. W: BCC (A2) ground state:

| | | | | |
|---|---|---|---|---|
| Space Group | | $Im\overline{3}m$ | $O_h^9$ | #229 |
| Pearson Symbol | | | cI2 | |
| $a$ , $b$ , $c$ | | 3.18934Å | 3.18934Å | 3.18934Å |
| $\alpha$ , $\beta$ , $\gamma$ | | 90° | 90° | 90° |
| Wyckoff Positions: | | | | |
| W | (2a) | 0 | 0 | 0 |
| Mesh | Γ | 38 × 38 × 38 | 1440 pts | in IBZ |
| Energy | | | -12.96121 eV | |

33. W: $\beta$-W (A15):

| | | | | |
|---|---|---|---|---|
| Space Group | | $Pm\overline{3}n$ | $O_h^3$ | #223 |
| Pearson Symbol | | | cP8 | |
| $a$ , $b$ , $c$ | | 5.08919Å | 5.08919Å | 5.08919Å |
| $\alpha$ , $\beta$ , $\gamma$ | | 90° | 90° | 90° |
| Wyckoff Positions: | | | | |
| W | (2a) | 1/2 | 1/2 | 1/2 |
| W | (6d) | 0 | 3/4 | 1/2 |
| Mesh | Γ | 17 × 17 × 17 | 1440 pts | in IBZ |
| Energy | | | -102.96141 eV | |

34. W: FCC (A1):

| | | | | |
|---|---|---|---|---|
| Space Group | $Fm\overline{3}m$ | | $O_h^5$ | #225 |
| Pearson Symbol | | | cF4 | |
| $a$ , $b$ , $c$ | | 4.04310Å | 4.04310Å | 4.04310Å |
| $\alpha$ , $\beta$ , $\gamma$ | | 90° | 90° | 90° |
| Wyckoff Positions: | | | | |
| W | (4a) | 0 | 0 | 0 |
| Mesh | Γ | $36 \times 36 \times 36$ | 1240 pts | in IBZ |
| Energy | | -12.48167 eV | | |

## IV. VDW-DF2 VAN DER WAALS FUNCTIONAL[9]

For comments on the individual phases see Sec. II.

1. $\alpha N_2$: High symmetry state:

| | | | | |
|---|---|---|---|---|
| Space Group | $Pa\overline{3}$ | | $T_h^6$ | #205 |
| Pearson Symbol | | | cP8 | |
| $a$ , $b$ , $c$ | | 5.51094Å | 5.51094Å | 5.51094Å |
| $\alpha$ , $\beta$ , $\gamma$ | | 90° | 90° | 90° |
| Wyckoff Positions: | | | | |
| N | (8c) | 0.55814 | 0.44186 | 0.94186 |
| Mesh | Γ | $8 \times 8 \times 8$ | 45 pts | in IBZ |
| Energy | | -70.50074 eV | | |

2. $\alpha N_2$: Low symmetry state:

| | | | | |
|---|---|---|---|---|
| Space Group | $P2_13$ | | $T^4$ | #198 |
| Pearson Symbol | | | cP8 | |
| $a$ , $b$ , $c$ | | 5.51064Å | 5.51064Å | 5.51064Å |
| $\alpha$ , $\beta$ , $\gamma$ | | 90° | 90° | 90° |
| Wyckoff Positions: | | | | |
| N | (4a) | 0.30714 | 0.19286 | 0.80714 |
| N | (4a) | 0.19086 | 0.30914 | 0.69086 |
| Mesh | M-P | $8 \times 8 \times 8$ | 24 pts | in IBZ |
| Energy | | -70.50068 eV | | |

3. $\beta N_2$:

| | | | | |
|---|---|---|---|---|
| Space Group | $P6_3/mmc$ | | $D_{6h}^4$ | #194 |
| Pearson Symbol | | | hP4 | |
| $a$ , $b$ , $c$ | | 3.37797Å | 3.37797Å | 8.17743Å |
| $\alpha$ , $\beta$ , $\gamma$ | | 90° | 90° | 120° |
| Wyckoff Positions: | | | | |
| N | (4f) | 1/3 | 2/3 | 0.18210 |
| Mesh | M-P | $16 \times 16 \times 12$ | 432 pts | in IBZ |
| Energy | | -35.16113 eV | | |

4. $\gamma N_2$:

| | | | | |
|---|---|---|---|---|
| Space Group | $P4_2/mnm$ | | $D_{4h}^{14}$ | #136 |
| Pearson Symbol | | | tP4 | |
| $a$ , $b$ , $c$ | | 5.00815Å | 5.00815Å | 3.40798Å |
| $\alpha$ , $\beta$ , $\gamma$ | | 90° | 90° | 90° |
| Wyckoff Positions: | | | | |
| N | (4f) | 0.07835 | 0.07835 | 0 |
| Mesh | M-P | $10 \times 10 \times 8$ | 60 pts | in IBZ |
| Energy | | -35.21670 eV | | |

5. $\varepsilon N_2$:

| | | | | |
|---|---|---|---|---|
| Space Group | $R\overline{3}c$ | | $D_{3d}^6$ | #167 |
| Pearson Symbol | | | hR48 | |
| $a$ , $b$ , $c$ | | 7.75359Å | 7.75359Å | 16.55181Å |
| $\alpha$ , $\beta$ , $\gamma$ | | 90° | 90° | 120° |
| Wyckoff Positions: | | | | |
| N | (12c) | 0 | 0 | 0.53352 |
| N | (36f) | 0.58164 | 0.89837 | 0.44951 |
| Mesh | M-P | $10 \times 10 \times 8$ | 60 pts | in IBZ |
| Energy | | -140.48436 eV | | |

6. $WN_4$ $ReP_4$: Again, we show the lowest energy state found so far:

| | | | | |
|---|---|---|---|---|
| Space Group | $Pbca$ | | $D_{2h}^{15}$ | #61 |
| Pearson Symbol | | | oP40 | |
| $a$ , $b$ , $c$ | | 14.11642Å | 6.41476Å | 9.54171 |
| $\alpha$ , $\beta$ , $\gamma$ | | 90° | 90° | 90° |
| Wyckoff Positions: | | | | |
| N | (8c) | 0.18177 | 0.99087 | 0.93130 |
| N | (8c) | 0.18027 | 0.49067 | 0.54699 |
| N | (8c) | 0.09200 | 0.99994 | 0.49938 |
| N | (8c) | 0.00007 | 0.24175 | 0.75379 |
| W | (8c) | 0.99967 | 0.00462 | 0.35394 |
| Mesh | Γ | $4 \times 6 \times 6$ | 48 pts | in IBZ |
| Energy | | -370.22509 eV | | |

7. $WN_3$ in Molybdite ($MoO_3$) structure:

| | | | | |
|---|---|---|---|---|
| Space Group | $Pnma$ | | $D_{2h}^{16}$ | #62 |
| Pearson Symbol | | | oP16 | |
| $a$ , $b$ , $c$ | | 19.58109Å | 4.11494Å | 2.98244Å |
| $\alpha$ , $\beta$ , $\gamma$ | | 90° | 90° | 90° |
| Wyckoff Positions: | | | | |
| N | (4c) | 0.54539 | 3/4 | 0.74058 |
| N | (4c) | 0.79496 | 3/4 | 0.21493 |
| N | (4c) | 0.60305 | 3/4 | 0.73618 |
| W | (4c) | 0.71166 | 3/4 | 0.71588 |
| Mesh | Γ | $6 \times 18 \times 24$ | 520 pts | in IBZ |
| Energy | | -147.38089 | | |

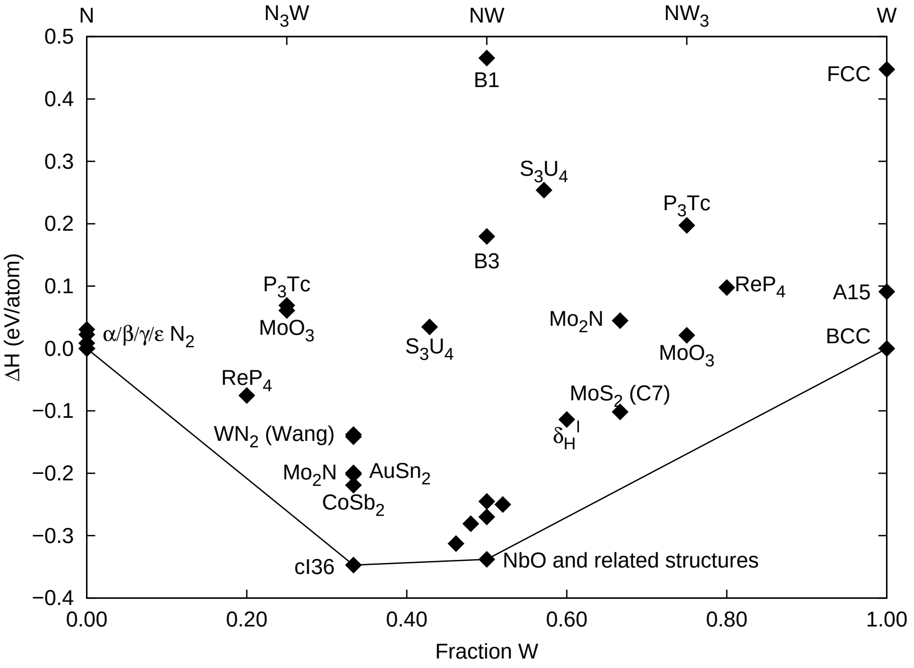


FIG. 3. Enthalpy per atom for $N_{1-x}W_x$ vdW-DF2 van der Waals functional approximation.

8. $WN_3$ in $P_3Tc$ structure:

| | | | | |
|---|---|---|---|---|
| Space Group | $Pnma$ | | $D_{2h}^{16}$ | #62 |
| Pearson Symbol | | | oP16 | |
| $a$ , $b$ , $c$ | | 13.01170Å | 3.03920Å | 5.14367Å |
| $\alpha$ , $\beta$ , $\gamma$ | | 90° | 90° | 90° |
| Wyckoff Positions: | | | | |
| N | (4c) | 0.52425 | 3/4 | 0.22113 |
| N | (4c) | 0.93420 | 3/4 | 0.32403 |
| N | (4c) | 0.76998 | 3/4 | 0.75149 |
| W | (4c) | 0.66742 | 3/4 | 0.03749 |
| Mesh | Γ | $4 \times 16 \times 8$ | 135 pts | in IBZ |
| Energy | | | -147.25028 | |

9. $WN_2$ in lower symmetry structure of Wang *et al.*:[15]

| | | | | |
|---|---|---|---|---|
| Space Group | $P\overline{6}m2$ | | $D_{3h}^{1}$ | #187 |
| Pearson Symbol | | | hP3 | |
| $a$ , $b$ , $c$ | | 2.99962Å | 2.99962Å | 3.97445Å |
| $\alpha$ , $\beta$ , $\gamma$ | | 90° | 90° | 120° |
| Wyckoff Positions: | | | | |
| N | (2g) | 0 | 0 | 0.18238 |
| W | (1d) | 1/3 | 2/3 | 1/2 |
| Mesh | Γ | $16 \times 16 \times 12$ | 210 pts | in IBZ |
| Energy | | | -28.68979 | |

10. $WN_2$ in higher symmetry structure of Wang *et al.*:[15]

| | | | | |
|---|---|---|---|---|
| Space Group | $P6_3/mmc$ | | $D_{6h}^{4}$ | #194 |
| Pearson Symbol | | | hP6 | |
| $a$ , $b$ , $c$ | | 3.00734Å | 3.00734Å | 7.89061Å |
| $\alpha$ , $\beta$ , $\gamma$ | | 90° | 90° | 120° |
| Wyckoff Positions: | | | | |
| N | (4e) | 0 | 0 | 0.09066 |
| W | (2d) | 1/3 | 2/3 | 3/4 |
| Mesh | Γ | $16 \times 16 \times 8$ | 150 pts | in IBZ |
| Energy | | | -27.39975 | |

11. $WN_2$ in $CoSb_2$ structure:

| | | | | |
|---|---|---|---|---|
| Space Group | $P2_1/c$ | | $C_{2h}^{5}$ | #14 |
| Pearson Symbol | | | mP12 | |
| $a$ , $b$ , $c$ | | 5.84252Å | 4.93943Å | 5.93500Å |
| $\alpha$ , $\beta$ , $\gamma$ | | 90° | 117.06754° | 90° |
| Wyckoff Positions: | | | | |
| N | (4e) | 0.40642 | 0.81372 | 0.09795 |
| N | (4e) | 0.08940 | 0.20214 | 0.39837 |
| W | (4e) | 0.23709 | 0.49323 | 0.29358 |
| Mesh | Γ | $8 \times 8 \times 4$ | 90 pts | in IBZ |
| Energy | | | -115.73069 | |

12. $WN_2$: constructed by removing 14 atoms from a 32 atom supercell of NaCl:

| | | | | |
|---|---|---|---|---|
| Space Group | | $Im\overline{3}m$ | $O_h^9$ | #229 |
| Pearson Symbol | | | cI36 | |
| $a$ , $b$ , $c$ | | 10.49032Å | 10.49032Å | 10.49032Å |
| $\alpha$ , $\beta$ , $\gamma$ | | 90° | 90° | 90° |
| Wyckoff Positions: | | | | |
| N | (24h) | 0 | 0.35447 | 0.35447 |
| W | (12d) | 0 | 1/4 | 1/2 |
| Mesh | Γ | 12 × 12 × 12 | 72 pts | in IBZ |
| Energy | | | -175.90495 | |

13. $WN_2$ in $AuSn_2$ structure:

| | | | | |
|---|---|---|---|---|
| Space Group | | $Pbca$ | $D_{2h}^{15}$ | #61 |
| Pearson Symbol | | | oP24 | |
| $a$ , $b$ , $c$ | | 9.97738Å | 5.03075Å | 5.28028Å |
| $\alpha$ , $\beta$ , $\gamma$ | | 90° | 90° | 90° |
| Wyckoff Positions: | | | | |
| N | (8c) | 0.96633 | 0.17410 | 0.67556 |
| N | (8c) | 0.71463 | 0.24276 | 0.57564 |
| W | (8c) | 0.64258 | 0.93919 | 0.82146 |
| Mesh | Γ | 8 × 8 × 4 | 75 pts | in IBZ |
| Energy | | | -230.99432 | |

14. $WN_2$ in $Mo_2N$ structure:

| | | | | |
|---|---|---|---|---|
| Space Group | | $I4_1/amd$ | $D_{4h}^{19}$ | #141 |
| Pearson Symbol | | | tI12 | |
| $a$ , $b$ , $c$ | | 3.84575Å | 3.84575Å | 10.80904Å |
| $\alpha$ , $\beta$ , $\gamma$ | | 90° | 90° | 90° |
| Wyckoff Positions: | | | | |
| N | (8e) | 1/2 | 1/4 | 0.92773 |
| W | (4b) | 1/2 | 1/4 | 0.12500 |
| Mesh | Γ | 12 × 12 × 20 | 667 pts | in IBZ |
| Energy | | | -57.76183 | |

15. $W_3N_4$ in $S_3U_4$ structure:

| | | | | |
|---|---|---|---|---|
| Space Group | | $Pm\overline{3}m$ | $O_h^1$ | #221 |
| Pearson Symbol | | | cP7 | |
| $a$ , $b$ , $c$ | | 4.31596Å | 4.31596Å | 4.31596Å |
| $\alpha$ , $\beta$ , $\gamma$ | | 90° | 90° | 90° |
| Wyckoff Positions: | | | | |
| N | (1a) | 0 | 0 | 0 |
| N | (3c) | 1/2 | 0 | 1/2 |
| W | (3d) | 0 | 1/2 | 0 |
| Mesh | Γ | 22 × 22 × 22 | 364 pts | in IBZ |
| Energy | | | -66.95987 eV | |

16. $W_6N_7$: constructed by removing 3 atoms from a 16 atom supercell of NaCl:

| | | | | |
|---|---|---|---|---|
| Space Group | | $Fm\overline{3}m$ | $O_h^5$ | #225 |
| Pearson Symbol | | | cF52 | |
| $a$ , $b$ , $c$ | | 8.51771Å | 8.51771Å | 8.51771Å |
| $\alpha$ , $\beta$ , $\gamma$ | | 90° | 90° | 90° |
| Wyckoff Positions: | | | | |
| N | (4b) | 1/2 | 1/2 | 1/2 |
| N | (24d) | 1/2 | 1/4 | 1/4 |
| W | (24e) | 0.22977 | 1/2 | 1/2 |
| Mesh | Γ | 12 × 12 × 12 | 72 pts | in IBZ |
| Energy | | | -129.65850 | |

17. $W_{12}N_{13}$: constructed by removing 7 atoms from a 32 atom supercell of NaCl:

| | | | | |
|---|---|---|---|---|
| Space Group | | $Im\overline{3}m$ | $O_h^9$ | #229 |
| Pearson Symbol | | | cI50 | |
| $a$ , $b$ , $c$ | | 8.46211Å | 8.46211Å | 8.46211Å |
| $\alpha$ , $\beta$ , $\gamma$ | | 90° | 90° | 90° |
| Wyckoff Positions: | | | | |
| N | (2a) | 0 | 0 | 0 |
| N | (24h) | 0 | 25070 | 0.25070 |
| W | (12d) | 0 | 1/4 | 1/2 |
| W | (12e) | 0.26499 | 0 | 0 |
| Mesh | Γ | 10 × 10 × 10 | 47 pts | in IBZ |
| Energy | | | -249.39171 | |

18. WN: NbO structure:

| | | | | |
|---|---|---|---|---|
| Space Group | | $Pm\overline{3}m$ | $O_h^1$ | #221 |
| Pearson Symbol | | | cP6 | |
| $a$ , $b$ , $c$ | | 4.20844Å | 4.20844Å | 4.20844Å |
| $\alpha$ , $\beta$ , $\gamma$ | | 90° | 90° | 90° |
| Wyckoff Positions: | | | | |
| N | (3c) | 1/2 | 0 | 1/2 |
| W | (3d) | 0 | 1/2 | 0 |
| Mesh | Γ | 20 × 20 × 20 | 286 pts | in IBZ |
| Energy | | | -60.41818 | |

19. WN: constructed by removing 4 atoms from a 16 atom body-centered tetragonal supercell of NaCl:

| | | | | |
|---|---|---|---|---|
| Space Group | | $I4mm$ | $C_{4v}^9$ | #107 |
| Pearson Symbol | | | tI24 | |
| $a$ , $b$ , $c$ | | 4.23932Å | 4.23932Å | 16.83746Å |
| $\alpha$ , $\beta$ , $\gamma$ | | 90° | 90° | 90° |
| Wyckoff Positions: | | | | |
| N | (2a) | 0 | 0 | 0.50379 |
| N | (2a) | 0 | 0 | 0.25101 |
| N | (4b) | 1/2 | 0 | 0.12202 |
| N | (4b) | 0 | 1/2 | 0.37361 |
| W | (2a) | 0 | 0 | 0.88287 |
| W | (2a) | 0 | 0 | 0.63508 |
| W | (4b) | 0 | 1/2 | 0.49590 |
| W | (4b) | 0 | 1/2 | 0.24710 |
| Mesh | Γ | 12 × 12 × 8 | 234 pts | in IBZ |
| Energy | | | -120.01844 | |

20. WN: constructed by removing 2 atoms from an 8 atom body-centered tetragonal supercell of NaCl:

| | | | | |
|---|---|---|---|---|
| Space Group | | $I4mm$ | $C_{4v}^9$ | #107 |
| Pearson Symbol | | | tI12 | |
| $a$ , $b$ , $c$ | | 4.23955Å | 4.23955Å | 8.38322Å |
| $\alpha$ , $\beta$ , $\gamma$ | | 90° | 90° | 90° |
| Wyckoff Positions: | | | | |
| N | (2a) | 0 | 0 | 0.98872 |
| N | (4b) | 0 | 1/2 | 0.25654 |
| W | (2a) | 0 | 0 | 0.72503 |
| W | (4b) | 1/2 | 0 | 0.01159 |
| Mesh | Γ | 20 × 20 × 20 | 641 pts | in IBZ |
| Energy | | | -59.86081 | |

21. WN: Cubic Zincblende (B3) structure:

| | | | | |
|---|---|---|---|---|
| Space Group | | $F\bar{4}3m$ | $T_d^2$ | #216 |
| Pearson Symbol | | | cF8 | |
| $a$ , $b$ , $c$ | | 4.77342Å | 4.77342Å | 4.77342Å |
| $\alpha$ , $\beta$ , $\gamma$ | | 90° | 90° | 90° |
| Wyckoff Positions: | | | | |
| N | (4a) | 0 | 0 | 0 |
| W | (4d) | 3/4 | 3/4 | 3/4 |
| Mesh | Γ | 20 × 20 × 20 | 256 pts | in IBZ |
| Energy | | | -19.10415 | |

22. WN: NaCl (B1) structure:

| | | | | |
|---|---|---|---|---|
| Space Group | | $Fm\bar{3}m$ | $O_h^5$ | #225 |
| Pearson Symbol | | | cF8 | |
| $a$ , $b$ , $c$ | | 4.47404Å | 4.47404Å | 4.47404Å |
| $\alpha$ , $\beta$ , $\gamma$ | | 90° | 90° | 90° |
| Wyckoff Positions: | | | | |
| N | (4a) | 0 | 0 | 0 |
| W | (4b) | 1/2 | 1/2 | 1/2 |
| Mesh | Γ | 24 × 24 × 24 | 413 pts | in IBZ |
| Energy | | | -18.53228 | |

23. $W_{13}N_{12}$: complementary structure to $W_{12}N_{13}$:

| | | | | |
|---|---|---|---|---|
| Space Group | | $Im\bar{3}m$ | $O_h^9$ | #229 |
| Pearson Symbol | | | cI50 | |
| $a$ , $b$ , $c$ | | 8.49968Å | 8.49968Å | 8.49968Å |
| $\alpha$ , $\beta$ , $\gamma$ | | 90° | 90° | 90° |
| Wyckoff Positions: | | | | |
| N | (12d) | 0 | 1/4 | 1/2 |
| N | (12e) | 0.26071 | 0 | 0 |
| W | (2a) | 0 | 0 | 0 |
| W | (24h) | 0 | 0.25349 | 0.25349 |
| Mesh | Γ | 10 × 10 × 10 | 47 pts | in IBZ |
| Energy | | | -250.46349 | |

24. $W_3N_4$ in $S_3U_4$ structure:

| | | | | |
|---|---|---|---|---|
| Space Group | | $Pm\bar{3}m$ | $O_h^1$ | #221 |
| Pearson Symbol | | | cP7 | |
| $a$ , $b$ , $c$ | | 4.39179Å | 4.39179Å | 4.39179Å |
| $\alpha$ , $\beta$ , $\gamma$ | | 90° | 90° | 90° |
| Wyckoff Positions: | | | | |
| N | (3d) | 0 | 1/2 | 0 |
| W | (1a) | 0 | 0 | 0 |
| W | (3c) | 1/2 | 0 | 1/2 |
| Mesh | Γ | 22 × 22 × 22 | 364 pts | in IBZ |
| Energy | | | -67.26306 eV | |

25. $W_3N_2$: hexagonal $\delta_H^I$ phase

| | | | | |
|---|---|---|---|---|
| Space Group | | $P6_3/mmc$ | $D_{6h}^4$ | #194 |
| Pearson Symbol | | | hP10 | |
| $a$ , $b$ , $c$ | | 2.96090Å | 2.96090Å | 16.26627Å |
| $\alpha$ , $\beta$ , $\gamma$ | | 90° | 90° | 120° |
| Wyckoff Positions: | | | | |
| N | (4f) | 2/3 | 1/3 | 0.16390 |
| W | (2c) | 2/3 | 1/3 | 3/4 |
| W | (4f) | 2/3 | 1/3 | 0.93195 |
| Mesh | Γ | 18 × 18 × 12 | 259 pts | in IBZ |
| Energy | | | -100.29345 | |

26. $W_2N$ in $MoS_2$ (C7) structure:

| | | | | |
|---|---|---|---|---|
| Space Group | $P6_3/mmc$ | | $D_{6h}^4$ | #194 |
| Pearson Symbol | | | hP6 | |
| $a$ , $b$ , $c$ | | 2.93256Å | 2.93256Å | 10.59144Å |
| $\alpha$ , $\beta$ , $\gamma$ | | 90° | 90° | 120° |
| Wyckoff Positions: | | | | |
| N | (2d) | 2/3 | 1/3 | 1/4 |
| W | (4f) | 2/3 | 1/3 | 0.88923 |
| Mesh | Γ | 16 × 16 × 4 | 90 pts | in IBZ |
| Energy | | | -60.83714 | |

27. $W_2N$ in $Mo_2N$ structure:

| | | | | |
|---|---|---|---|---|
| Space Group | $I4_1/amd$ | | $D_{4h}^{19}$ | #141 |
| Pearson Symbol | | | tI12 | |
| $a$ , $b$ , $c$ | | 4.41275Å | 4.41275Å | 8.08133Å |
| $\alpha$ , $\beta$ , $\gamma$ | | 90° | 90° | 90° |
| Wyckoff Positions: | | | | |
| N | (4a) | 0 | 3/4 | 0.12500 |
| W | (8e) | 1/2 | 1/4 | 0.89469 |
| Mesh | Γ | 10 × 10 × 18 | 474 pts | in IBZ |
| Energy | | | -59.95971 | |

28. $W_2N$: Complementary structure to cubic $WN_2$ structure with space group $Im\overline{3}m$:

| | | | | |
|---|---|---|---|---|
| Space Group | $Im\overline{3}m$ | | $O_h^9$ | #229 |
| Pearson Symbol | | | cI36 | |
| $a$ , $b$ , $c$ | | 8.06722Å | 8.06722Å | 8.06722Å |
| $\alpha$ , $\beta$ , $\gamma$ | | 90° | 90° | 90° |
| Wyckoff Positions: | | | | |
| N | (12d) | 0 | 1/4 | 1/2 |
| W | (24h) | 0 | 0.24668 | 0.24668 |
| Mesh | Γ | 12 × 12 × 12 | 72 pts | in IBZ |
| Energy | | | -199.10483 | |

29. $W_3N$: $MoO_3$ structure. Again, it relaxes to a higher symmetry structure:

| | | | | |
|---|---|---|---|---|
| Space Group | $Cmcm$ | | $D_{2h}^{17}$ | #63 |
| Pearson Symbol | | | oC16 | |
| $a$ , $b$ , $c$ | | 4.32374Å | 12.30623Å | 4.29525Å |
| $\alpha$ , $\beta$ , $\gamma$ | | 90° | 90° | 90° |
| Wyckoff Positions: | | | | |
| N | (4c) | 1/2 | 0.42369 | 3/4 |
| W | (4c) | 1/2 | 0.60414 | 3/4 |
| W | (4c) | 1/2 | 0.91430 | 3/4 |
| W | (4c) | 1/2 | 0.24403 | 3/4 |
| Mesh | Γ | 12 × 12 × 16 | 387 pts | in IBZ |
| Energy | | | -81.36195 | |

30. $W_3N$: $P_3Tc$ structure:

| | | | | |
|---|---|---|---|---|
| Space Group | $Pnma$ | | $D_{2h}^{16}$ | #62 |
| Pearson Symbol | | | oP16 | |
| $a$ , $b$ , $c$ | | 16.53087Å | 2.89162Å | 4.87654Å |
| $\alpha$ , $\beta$ , $\gamma$ | | 90° | 90° | 90° |
| Wyckoff Positions: | | | | |
| N | (4c) | 0.66385 | 3/4 | 0.97499 |
| W | (4c) | 0.55241 | 3/4 | 0.73903 |
| W | (4c) | 0.89019 | 3/4 | 0.76908 |
| W | (4c) | 0.77087 | 3/4 | 0.21742 |
| Mesh | Γ | 4 × 14 × 10 | 144 pts | in IBZ |
| Energy | | | -159.90177 | |

31. $W_4N$: $ReP_4$ structure:

| | | | | |
|---|---|---|---|---|
| Space Group | $Pbca$ | | $D_{2h}^{15}$ | #61 |
| Pearson Symbol | | | oP40 | |
| $a$ , $b$ , $c$ | | 11.95901Å | 5.19585Å | 9.61003Å |
| $\alpha$ , $\beta$ , $\gamma$ | | 90° | 90° | 90° |
| Wyckoff Positions: | | | | |
| N | (8c) | 0.06028 | 0.92374 | 0.38005 |
| W | (8c) | 0.19039 | 0.11025 | 0.25758 |
| W | (8c) | 0.18620 | 0.74775 | 0.50595 |
| W | (8c) | 0.07170 | 0.27888 | 0.50422 |
| W | (8c) | 0.07063 | 0.59124 | 0.24724 |
| Mesh | Γ | 4 × 8 × 4 | 45 pts | in IBZ |
| Energy | | | -407.41227 | |

32. W: BCC (A2) ground state:

| | | | | |
|---|---|---|---|---|
| Space Group | | $Im\overline{3}m$ | $O_h^9$ | #229 |
| Pearson Symbol | | | cI2 | |
| $a$ , $b$ , $c$ | | 3.25029Å | 3.25029Å | 3.25029Å |
| $\alpha$ , $\beta$ , $\gamma$ | | 90° | 90° | 90° |
| Wyckoff Positions: | | | | |
| W | (2a) | 0 | 0 | 0 |
| Mesh | Γ | 32 × 32 × 32 | 897 pts | in IBZ |
| Energy | | | -10.65066 | |

33. W: $\beta$-W (A15):

| | | | | |
|---|---|---|---|---|
| Space Group | | $Pm\overline{3}n$ | $O_h^3$ | #223 |
| Pearson Symbol | | | cP8 | |
| $a$ , $b$ , $c$ | | 5.18500Å | 5.18500Å | 5.18500Å |
| $\alpha$ , $\beta$ , $\gamma$ | | 90° | 90° | 90° |
| Wyckoff Positions: | | | | |
| W | (2a) | 1/2 | 1/2 | 1/2 |
| W | (6d) | 0 | 1/4 | 1/2 |
| Mesh | Γ | 12 × 12 × 12 | 84 pts | in IBZ |
| Energy | | | -84.47732 | |

34. W: FCC (A1):

| | | | | |
|---|---|---|---|---|
| Space Group | | $Fm\overline{3}m$ | $O_h^5$ | #225 |
| Pearson Symbol | | | cF4 | |
| $a$ , $b$ , $c$ | | 4.12107Å | 4.12107Å | 4.12107Å |
| $\alpha$ , $\beta$ , $\gamma$ | | 90° | 90° | 90° |
| Wyckoff Positions: | | | | |
| W | (4a) | 0 | 0 | 0 |
| Mesh | Γ | 32 × 32 × 32 | 897 pts | in IBZ |
| Energy | | | -10.20318 | |

* michael.mehl@nrl.navy.mil
† stefano@duke.edu

1 G. Kresse and J. Hafner, Phys. Rev. B **48**, 13115 (1993).
2 G. Kresse and J. Hafner, Phys. Rev. B **49**, 14251 (1994).
3 G. Kresse, Ph.D. thesis, Technische Universität Wien, Vienna (1993).
4 P. E. Blöchl, Phys. Rev. B **50**, 17953 (1994).
5 G. Kresse and D. Joubert, Phys. Rev. B **59**, 1758 (1999).
6 S. Curtarolo, W. Setyawan, G. L. W. Hart, M. Jahnatek, R. V. Chepulskii, R. H. Taylor, S. Wang, J. Xue, K. Yang, O. Levy, M. Mehl, H. T. Stokes, D. O. Demchenko, and D. Morgan, Comp. Mat. Sci. **58**, 218–226 (2012).
7 S. Curtarolo, G. L. W. Hart, M. Buongiorno Nardelli, N. Mingo, S. Sanvito, and O. Levy, Nat. Mater. **12**, 191–201 (2013).
8 S. Curtarolo, W. Setyawan, S. Wang, J. Xue, K. Yang, R. H. Taylor, L. J. Nelson, G. L. W. Hart, S. Sanvito, M. Buongiorno Nardelli, N. Mingo, and O. Levy, Comp. Mat. Sci. **58**, 227–235 (2012).
9 M. Dion, H. Rydberg, E. Schroder, D. C. Langreth, and B. I. Lundqvist, Phys. Rev. Lett. **92**, 246401 (pages 4) (2004).
10 J. Klimeš, D. R. Bowler, and A. Michaelides, J. Phys.: Condens. Matt. **22**, 022201 (2010).
11 J. Klimeš, D. R. Bowler, and A. Michaelides, Phys. Rev. B **83**, 195131 (2011).
12 J. P. Perdew, K. Burke, and M. Ernzerhof, Phys. Rev. Lett. **77**, 3865 (1996).
13 H. J. Monkhorst and J. D. Pack, Phys. Rev. B **13**, 5188 (1976).
14 S. Aydina, Y. O. Ciftci, and A. Tatar, J. Mater. Res. **27**, 1705 (2012).
15 H. Wang, Q. Li, Y. Li, Y. Xu, T. Cui, A. R. Oganov, and Y. Ma, Phys. Rev. B **79**, 132109 (pages 4) (2009).
16 M. Zumbusch, Z. Anorg. Allg. Chem. **243**, 322 (1940).
17 V. I. Khitrova and Z. G. Pinsker, Sov. Phys. Crystallogr. **6**, 712 (1962).
